# Supplementary material for: Leveraging Multimodal Features and Item-level User Feedback for Bundle Construction
Source: arXiv:2310.18770 source file (2023-10-28)
Supplement: Supplementary file 1 [file 7_appendix.tex]

\newpage
\appendix
\section{Appendix} \label{sec:app}
